# Supplementary material for: Digital cities and the spread of COVID-19: characterizing the impact of non-pharmaceutical interventions in five cities in Spain
Source: arXiv:2212.06659 source file (2022-12-13)
Supplement: Supplementary file 1 [file Rodriguez_Aleta_Moreno_Supplementary.pdf]

# Digital cities and the spread of COVID-19: characterizing the impact of non-pharmaceutical interventions in five cities in Spain

Jorge P. Rodríguez, Alberto Aleta, Yamir Moreno

SUPPLEMENTARY MATERIAL

## **DIGITAL CITIES: DATA SOURCES**

### **Data available from scientific literature**

-Contact matrices for 152 countries (data obtained: Spain, other locations, used for inferring community layer):

<https://journals.plos.org/ploscompbiol/article?id=10.1371/journal.pcbi.1005697#sec020>

### **Data available from national sources**

-Instituto Nacional de Estadística, population by age and sex, home sizes and home structure, at district level:

<https://www.ine.es/censos2011/tablas/Inicio.do>

-Registered students at university, per degree and university:

<https://www.ciencia.gob.es/portal/site/MICINN/menuitem.7eeac5cd345b4f34f09dfd1001432ea0/?vgnnextoid=0930dd449de8b610VgnVCM1000001d04140aRCRD>

-Statistics of registered students at university, BsC (data obtained: ages):

[http://estadisticas.mecd.gob.es/EducaDynPx/educabase/index.htm?type=pcaxis&path=/Universitaria/Alumnado/Nueva\\_Estructura/GradoCiclo/Matriculados/&file=pcaxis](http://estadisticas.mecd.gob.es/EducaDynPx/educabase/index.htm?type=pcaxis&path=/Universitaria/Alumnado/Nueva_Estructura/GradoCiclo/Matriculados/&file=pcaxis)

-Statistics of registered students at university, MsC (data obtained: ages):

[http://estadisticas.mecd.gob.es/EducaDynPx/educabase/index.htm?type=pcaxis&path=/Universitaria/Alumnado/Nueva\\_Estructura/Master/Matriculados/&file=pcaxis](http://estadisticas.mecd.gob.es/EducaDynPx/educabase/index.htm?type=pcaxis&path=/Universitaria/Alumnado/Nueva_Estructura/Master/Matriculados/&file=pcaxis)

-Age of registered students at job training programs (used data from course 2018-2019):

<http://estadisticas.mecd.gob.es/EducaDynPx/educabase/index.htm?type=pcaxis&path=/Educacion/Alumnado/Matriculado/2018-2019RD/RGCiclosFP&file=pcaxis&l=s0>

-Private request to the Ministry of Universities (Spain) on the number of registered students at university per municipality (BsC and MsC).

-Instituto Nacional de Estadística, number of companies per region and number of employees:

<https://www.ine.es/jaxiT3/Tabla.htm?t=298&L=0>

-Instituto Nacional de Estadística, national employment survey, information at municipality level (using data at the first term of 2019):

[https://www.ine.es/dyngs/INEbase/es/operacion.htm?c=Estadistica\\_C&cid=1254736176918&menu=resultados&idp=1254735976595](https://www.ine.es/dyngs/INEbase/es/operacion.htm?c=Estadistica_C&cid=1254736176918&menu=resultados&idp=1254735976595)

-Number of affiliated employees to the National Social Security, by municipality (using data at the last day of January 2019):

<https://www.seg-social.es/wps/portal/wss/internet/EstadisticasPresupuestosEstudios/Estadisticas/EST8/EST167/21b04ced-f0f1-4bb9-9662-0437a6f9934e/29f824da-afbf-4af2-aa3e-9c8751e86991>

-Instituto Nacional de Estadística, age and gender of residents in nursing homes:

<https://www.ine.es/jaxi/Tabla.htm?path=/t20/e244/colectivos/p02/10/&file=02005.px&L=0>

-Envejecimiento en red (CSIC), number of places and nursing homes per municipality:

<http://envejecimiento.csic.es/documentos/recursos/residencias/>

### **Data available from regional/local sources**

#### **1. Barcelona**

-Population by age and sex, at district level:

<https://www.bcn.cat/estadistica/castella/dades/tpob/pad/padro/a2020/edat/edatq03.htm>

<https://www.bcn.cat/estadistica/castella/dades/tpob/pad/padro/a2020/edat/edatq04.htm>

-Number of school students, number of units and number of centres at district level, data obtained for course 2019-2020, for different levels:

<https://educacio.gencat.cat/ca/departament/estadistiques/estadistiques-ensenyament/cursos-anteriors/curs-2019-2020/>

#### **2. Valencia**

-Population by age and sex, at district level:

<http://www.valencia.es/ayuntamiento/catalogo.nsf/IndiceAnuario?readForm&lang=1&capitulo=2&tema=2&bdOrigen=ayuntamiento/estadistica.nsf&idApoyo=58FB3C7A3D56E414C1257DD40057EB6C>

-Students registered in each unit (per level) in school programs, by centre:

<https://dadesobertes.gva.es/es/dataset/edu-alu-gen-2020>

-Students registered in each unit in job training programs, by centre:

<https://dadesobertes.gva.es/es/dataset/edu-alu-fp-2020>

-List of scholar centres, including their geographical coordinates (updated 21 September 2020):

<http://www.ceice.gva.es/es/web/centros-docentes/descarga-base-de-datos>

### 3. Seville

-Population by age and sex, at district resolution:

<https://www.sevilla.org/servicios/servicio-de-estadistica/datos-estadisticos/explotacion-estadistica-padron#autotoc-item-autotoc-0>

-Number of students, number of units and number of centres per level per municipality (3. Sociedad, 3.1 Enseñanza y formación):

[https://www.juntadeandalucia.es/institutodeestadisticaycartografia/badea/informe/anual?CodOper=b3\\_151&idNode=23204](https://www.juntadeandalucia.es/institutodeestadisticaycartografia/badea/informe/anual?CodOper=b3_151&idNode=23204)

-List of scholar centres, including their geographical coordinates:

<https://www.juntadeandalucia.es/datosabiertos/portal/dataset/directorio-de-centros-docentes-de-andalucia#csv>

### 4. Zaragoza

-Number of students, number of units and number of centres, per level per municipality:

<https://www.aragon.es/-/enseanzas-de-regimen-general>

-List of scholar centres, including their geographical coordinates:

<https://opendata.aragon.es/datos/catalogo/dataset/directorio-de-centros-educativos-de-aragon>

### 5. Murcia

-Population by age and sex, at section resolution (districts are composed by sections):

[https://econet.carm.es/web/crem/inicio/-/crem/sicrem/PU\\_padron/p20/sec23\\_sec24\\_31.html](https://econet.carm.es/web/crem/inicio/-/crem/sicrem/PU_padron/p20/sec23_sec24_31.html)

[https://econet.carm.es/web/crem/inicio/-/crem/sicrem/PU\\_padron/p20/sec24\\_sec25\\_31.html](https://econet.carm.es/web/crem/inicio/-/crem/sicrem/PU_padron/p20/sec24_sec25_31.html)

-Number of students, number of units and number of centres, per level per municipality:

[https://econet.carm.es/web/crem/inicio/-/crem/sicrem/PU\\_EDUCNOUNIV/Indice2016.html](https://econet.carm.es/web/crem/inicio/-/crem/sicrem/PU_EDUCNOUNIV/Indice2016.html)

-List of scholar centres, including their geographical coordinates:

[https://murciaencifras-com.carto.com/tables/centros\\_educativos\\_1/public](https://murciaencifras-com.carto.com/tables/centros_educativos_1/public)
